# Supplementary material for: Unsupervised Robust Cross-Lingual Entity Alignment via Neighbor Triple Matching with Entity and Relation Texts
Source: arXiv:2407.15588 source file (2025-02-12)
Supplement: Supplementary file 1 [file bak-060appendix.tex]

\section{Overall Process of \proposedpp}
\label{sec:pseudocode}
Algorithm~\ref{alg:eralign} outlines the comprehensive pseudo-code for \proposedpp. 
The algorithm initiates by constructing dual graphs for both the source and target KGs (Line 1), and then, it derives the initial alignment matrices for entities and relations by solving the OT problem using the Sinkhorn algorithm (Lines 2--3).
The iterative refinement process follows, updating the initial alignment results through the fusion of both alignment scores based on neighbor triple matching (Line 4), thereby obtaining the final alignment results (Line 5). 
In the verification step, \proposedpp assesses the confidence and consistency scores for each entity in the source KG (Lines 6--7) and assembles the set of entities slated for verification (Line 8). 
For each entity in $\mathcal{E}^{ver}$, the algorithm identifies the Top-$K$ candidate entities for alignment from the target KG (Line 9) and reorders their alignment ranks based on the semantic textual similarities of the entities' neighbor triples (Line 10).

\begin{algorithm}
\caption{The overall process of \proposedpp}
\label{alg:eralign}
\SetAlgoLined
\textbf{Input}: The source and target KGs $\mathcal{G}_S=(\mathcal{E}_S, \mathcal{R}_S, \mathcal{T}_S)$ and $\mathcal{G}_T=(\mathcal{E}_T, \mathcal{R}_T, \mathcal{T}_T)$, the PLM fine-tuned for STS $f_\phi$\\
% \textbf{Output}: 
% The entity-entity alignment matrix $\widehat{\bm{S}}^{ent}$\\
\vspace{5pt}
\tcp{\small Step 1: Dual alignment of entities and relations}
\nl Construct the dual graphs $\widebar{\mathcal{G}}_S$ and $\widebar{\mathcal{G}}_T$ from ${\mathcal{G}}_S$ and ${\mathcal{G}}_T$ \\
\nl Obtain the entity alignment matrix $\widehat{\bm{X}}^{ent}$ by Eq.~\eqref{eq:seuoriginal}, \eqref{eq:seuentfinal} \\
\nl Obtain the relation alignment matrix $\widehat{\bm{X}}^{rel}$ by Eq.~\eqref{eq:seudual}, \eqref{eq:seurelfinal}\\\vspace{5pt}
\tcp{\small Step 2: Iterative refinement of dual alignment}
\For{$n\in\{1,\ldots,N\}$}
{
\nl Update the alignment matrices ${\bm{S}}_{n}^{ent}$, ${\bm{S}}_{n}^{rel}$ by Eq.~\eqref{eq:fusionent}, \eqref{eq:fusionrel}
}
\nl Obtain the alignment matrices $\widehat{\bm{S}}^{ent}$, $\widehat{\bm{S}}^{rel}$ by Eq.~\eqref{eq:entfinal}, \eqref{eq:relfinal}\\
\vspace{5pt}
\tcp{\small Step 3: Erroneous alignment verification}
\For{$i\in\mathcal{E}_S$}{
\nl Calculate $\textbf{Conf}(i)=\max([\widehat{\bm{S}}^{ent}]{i:})$ \\
\nl Calculate $\textbf{Cons}(i) = \text{cos}([\widehat{\bm{X}}^{ent}]_{i:}, [\widehat{\bm{S}}^{ent}]_{i:})$
}
\nl Collect the entity set for verification $\mathcal{E}^{ver}=\{i|\textbf{Conf}(i)<\theta_{conf} \lor \textbf{Cons}(i)<\theta_{cons}, \forall i\in\mathcal{E}_S\}$ \\
\For{$i\in\mathcal{E}^{ver}$}{
\nl Obtain the candidate entities $\text{Cand}(i)=\text{Top-}K([\widehat{\bm{S}}^{ent}]_{i:})$ \\
\nl Rerank the entities in Cand$(i)$ with $f_\phi$ by Eq.~\eqref{eq:verfsrc}, \eqref{eq:verftgt}
}
\end{algorithm}

\section{Template for Triple Linearization}
\label{sec:template}
To linearize an entity's relation triples, we employ a straightforward text template that succinctly summarizes relevant knowledge, focusing on the entity.
\begin{equation}
\begin{split}
    Z_S(i) &= \text{``}[\texttt{Entity} \text{ } i], \text{which ''} \\
    &+ \Vert_{(i, p, i')\in\mathcal{T}'} \text{``}[\texttt{Relation} \text{ } p] \text{ is } [\texttt{Entity} \text{ } i']\text{, ''}
\end{split}
\end{equation}
For instance, in the DBP\textsubscript{EN} KG, the entity ``Football League One'' can be represented through linearized text based on its neighbor triples:
``Football League One, which relegation is Football League Championship, promotion is Football League Championship, promotion is Football League Two, relegation is Football League Two, league is Sheffield United F.C..''.
An alternative approach to linearization involves employing language models fine-tuned to transform a subgraph (e.g., 1-hop triple knowledge) into plausible text~\cite{graph2text}.
This avenue is left for future exploration.

\section{Erroneous Alignment Verification}
\label{sec:verfmatrix}
For in-depth analyses on the efficacy of our verification step, we thoroughly examine the verification matrix summarizing the counts of correctly/incorrectly aligned entity pairs before and after the correction process in Table~\ref{tbl:verfmat}. 
Entities labeled as ``non-detected'' are excluded from correction (i.e., $\notin\mathcal{E}^{ver}$), and entities classified as ``non-corrected'' do not pass the cross-verification, resulting in no adjustments to the ranked list.
In the case of both non-detected and non-corrected entities, where no modifications were made, we discover that most of them are actually challenging to accurately rectify by using only semantic textual relevance of entities' neighbor triples;
this difficulty mostly arises from structural disparities between the source and target KGs.
In the case of corrected alignments, over 90\% of corrections result in accurate alignments (i.e., $\bm{\times\rightarrow\checkmark}$ and $\bm{\checkmark\rightarrow\checkmark}$), thereby significantly improving overall alignment accuracy.
Furthermore, the effectiveness of our verification step becomes particularly pronounced as the noise level increases, strongly indicating that the additional verification substantially enhances alignment accuracy in the presence of textual noise.





\begin{table}[t]
\caption{Verification matrices illustrating the number of corrected erroneous alignments by \proposedpp, Dataset: \dbpzh. Entities labeled as ``non-detected'' are not considered for correction (i.e., $\notin\mathcal{E}^{ver}$), and entities classified as ``non-corrected'' fail the cross-verification, resulting in no adjustments to the ranked list.}
    \label{tbl:verfmat}
    \centering
    \resizebox{0.99\linewidth}{!}{
        \begin{tabular}{ccPPPP}
            \toprule
            & & \multicolumn{3}{c}{\textbf{Detected}} & {\textbf{Non-Detected}} \\\cmidrule(lr){3-5}\cmidrule(lr){6-6}
            & & \multicolumn{2}{c}{\textbf{Before Correction}} & \multirow{2}{*}{\makecell{Non-\\Corrected}} & \multirow{2}{*}{\makecell{Non-\\Detected}} \\
            % \cmidrule{3-4}
            & & Wrong & Correct & & \\
            \midrule
            % \cmidrule(lr){3-4}\cmidrule(lr){5-5}\cmidrule(lr){6-6}
            
            \multirow{6.5}{*}{\rotatebox[origin=c]{90}{\textbf{Noise 0\%}}} & \multirow{3}{*}{\rotatebox[origin=c]{90}{{Wrong}}} 

            & $\bm{\times \rightarrow \times}$ & $\bm{\checkmark \rightarrow \times}$ & $\bm{\times (\rightarrow \times)}$ & $\bm{\times (\rightarrow \times)}$  \\
            & & 26 & 43 & 505 & 262 \\
            & & (2.9\%) & (4.7\%) & &  \\
            \cmidrule(l){2-6}
            
            & \multirow{3}{*}{\rotatebox[origin=c]{90}{{Correct}}} 
            
            & $\bm{\times \rightarrow \checkmark}$ & $\bm{\checkmark \rightarrow \checkmark}$ & $\bm{\checkmark (\rightarrow \checkmark)}$ & $\bm{\checkmark (\rightarrow \checkmark)}$ \\
            & & 88 & 753 & 1,494 & 11,910 \\
            & & (9.7\%) & (82.7\%) & &  \\
            
            \midrule
            \multirow{6.5}{*}{\rotatebox[origin=c]{90}{\textbf{Noise 10\%}}} & \multirow{3}{*}{\rotatebox[origin=c]{90}{{Wrong}}} 

            & $\bm{\times \rightarrow \times}$ & $\bm{\checkmark \rightarrow \times}$ & $\bm{\times (\rightarrow \times)}$ & $\bm{\times (\rightarrow \times)}$  \\
            & & 33 & 44 & 534 & 370 \\
            & & (2.9\%) & (3.8\%) & &  \\
            \cmidrule(l){2-6}
            
            & \multirow{3}{*}{\rotatebox[origin=c]{90}{{Correct}}} 
            
            & $\bm{\times \rightarrow \checkmark}$ & $\bm{\checkmark \rightarrow \checkmark}$ & $\bm{\checkmark (\rightarrow \checkmark)}$ & $\bm{\checkmark (\rightarrow \checkmark)}$ \\
            & & 180 & 894 & 1,149 & 11,796 \\
            & & (15.6\%) & (77.7\%) & &  \\
            
            \midrule
            % \cmidrule(lr){3-4}\cmidrule(lr){5-5}\cmidrule(lr){6-6}
            
            \multirow{6.5}{*}{\rotatebox[origin=c]{90}{\textbf{Noise 20\%}}} & \multirow{3}{*}{\rotatebox[origin=c]{90}{{Wrong}}} 

            & $\bm{\times \rightarrow \times}$ & $\bm{\checkmark \rightarrow \times}$ & $\bm{\times (\rightarrow \times)}$ & $\bm{\times (\rightarrow \times)}$  \\
            & & 38 & 48 & 568 & 512 \\
            & & (2.8\%) & (3.5\%) & &  \\
            \cmidrule(l){2-6}
            
            & \multirow{3}{*}{\rotatebox[origin=c]{90}{{Correct}}} 
            
            & $\bm{\times \rightarrow \checkmark}$ & $\bm{\checkmark \rightarrow \checkmark}$ & $\bm{\checkmark (\rightarrow \checkmark)}$ & $\bm{\checkmark (\rightarrow \checkmark)}$ \\
            & & 256 & 1,026 & 882 & 11,670 \\
            & & (18.7\%) & (75.0\%) & &  \\
            \bottomrule
        \end{tabular}
    }
\end{table}

\section{Textual Noise Simulation in KGs}
\label{sec:noise}
To assess the robustness of \proposed and \proposedpp in the presence of textual feature noise (discussed in Section~\ref{subsubsec:noise}), we conduct experiments simulating various types of text translation errors that commonly manifest as noise. 
We focus on three distinct categories of textual noise, outlined as follows:
\begin{itemize}
    \item \textbf{Phonetic errors}: 
    These errors involve variations in the representation of words based on their phonetic similarity. 
    For instance, substitutions like
    `intu'/`into', `o'/`oe', `li'/`ri', `ty'/`ti', `cu'/`ka', `ca'/`ka', `ar'/`al', `tic'/`th', `se'/`th', `nes'/`nais', `ud'/`ade', `Ji'/`Gi', `fi'/`fy', `ps'/`pus', `er'/`ar', `our'/`ur', `ar'/`ur', `la'/`ra', `ei'/`ee', `ny'/`ni', `ew'/`ou', `ar'/`or', `or'/`ol', `ol'/`oul', `ry'/`ly', `wi'/`wy', or `ic'/`ik'
    are considered phonetic errors.

    \item \textbf{Missing characters}: 
    This type of error occurs when certain characters are omitted from a word. 
    Examples include instances where `-s', `-e', or ` ' (blank) are missing.
    
    \item \textbf{Attached characters}:
    Attached characters refer to errors where additional characters are affixed to a word. 
    For example, errors such as `-s' or `-e' being added to a word fall into this category.
\end{itemize}


\section{Compatibility of \proposed with \eva}
\label{sec:application}
To investigate the compatibility of \proposed (in Section~\ref{subsubsec:application}), we utilize the entity-level and relation-level alignment scores, initially obtained by \eva~\cite{eva} which is a self-supervised cross-lingual EA method.
Since \eva is originally designed for unsupervised multi-modality entity alignment (MMEA),
it leverages the similarity of visual information of entities to generate a pseudo seed alignment (i.e., visual pivot dictionary) used for model training.
This work only focuses on textual and structural information, and thus we tailor \eva for using the textual information of nodes (i.e., entity name for original KGs and relation name for dual KGs) instead of their visual information, to collect pseudo seed alignment.
We combine \sbert (as semantic features) and Bigram (as lexical features) to obtain final textual embeddings.

% initial seeds
For initial seeds, we collect top-$k$ entity pairs based on the similarity of their textual embeddings.
To keep the initial seeds small, we set $k$ to 10\% of the number of ground-truth pairs.
Specifically, the number of initial seeds for entity alignment is 1500, while those for relation alignment are 89 (\dbpzh) and 58 (\dbpja).
% Due to the absence of officially available ground-truth relation pairs, we set pairs with matching names before preprocessing, leading in different quantities across datasets.

% training
We use 2-layer graph convolution networks (GCNs) with input, hidden, and output dimension of 128.
As the number of initial seeds are small, we make \eva adopt the iterative learning (IL) strategy. 
The IL method expands the training set by updating the candidate set during training and merging it into the training set at certain epochs.
The training process takes the total epochs of 1000, and IL is applied after the first 500 epochs.
The candidate set is updated every 10 epochs and merged into training set every 10 updates (i.e., 100 epochs).
For optimization, we use AdamW~\cite{adamw} as the optimizer with a learning rate of $5e-4$ and weight decay of $1e-2$.
The output alignment scores from \eva is considered as the initial alignment scores (Step 1) within our \proposed framework in Section~\ref{subsubsec:application}.
Table~\ref{tbl:eva} reports the accuracy of \eva in terms of both the entity-level and relation-level alignment between source and target KGs.

\begin{table}[t]
\caption{The accuracy of initial alignment scores}
    \label{tbl:eva}
    \centering
    \resizebox{0.99\linewidth}{!}{%
    \begin{tabular}{cccccccc}
        \toprule
        
        \multicolumn{2}{c}{\multirow{2.5}{*}{\textbf{Alignment Score}}}
        & \multicolumn{3}{c}{\textbf{\dbpzh}} 
        & \multicolumn{3}{c}{\textbf{\dbpja}} \\ 
        \cmidrule(lr){3-5}\cmidrule(lr){6-8}

        & 
        & \small H@1 & \small H@10 & \small MRR
        & \small H@1 & \small H@10 & \small MRR\\ 
        \midrule

        % \ Entity
        \multirow{2}{*}{\rotatebox[origin=c]{0}{\small \eva}}
        & Entity-level
        & {0.828} & {0.923} & {0.864}
        & {0.917} & {0.974} & {0.979} \\
        & Relation-level
        & {0.965} & {0.997} & {0.980}
        & {0.935} & {1.000} & {0.966} \\
        \midrule

        \multirow{2}{*}{\rotatebox[origin=c]{0}{\small \seu}}
        & Entity-level
        & {0.929} & {0.972} & {0.945}
        & {0.975} & {0.994} & {0.982} \\
        & Relation-level
        & {0.992} & {1.000} & {0.996}
        & {0.983} & {1.000} & {0.990} \\


       \bottomrule
    \end{tabular}
    }
\end{table}
